# Supplementary material for: The Large Synoptic Survey Telescope as a Near-Earth Object Discovery Machine
Source: arXiv:1711.10621 source file (2017-11-29)
Supplement: Supplementary file 1 [file appendix_fallback_strategies.tex]

\section{Fallback survey strategies}\label{sec:AppFallback}

To investigate the effects of requiring triplets or quads of visits within a single night as part of the discovery criteria, instead of simply pairs, two additional simulated surveys were run where the WFD (but not the NES) requested visits in sequences of three or four, instead of just pairs. It is important to note that due to the behavior of the OpSim software, it is frequently the case that more than the requested minimum number of visits are received in a particular field on a given night. That is, even in the baseline minion\_1016 run, which requested pairs of visits in each night for the WFD and NES, it is often the case that three or four visits were obtained despite the smaller request. Thus, these additional runs provide an indication of the trade-offs in coverage and completeness that result from requesting more visits per field, per night, but the effects would be more pronounced if this behavior of the software did not exist. The simulated surveys enigma\_1281 and enigma\_1282 are the result of requesting triples and quads in the WFD proposal, with 2,052,029 and 2,033,431 WFD visits in these runs, respectively.

Effects of pairs vs triples vs quads - minion\_1016 vs enigma\_1281 vs enigma\_1282.
